# Supplementary material for: Root Cause Analysis for Microservice System based on Causal Inference: How Far Are We?
Source: arXiv:2408.13729 source file (2024-09-08)
Supplement: Supplementary file 1 [file 7.appendix.tex]

\section{More Information about Causal Discovery Methods for Time Series} \label{sec:app-causal-discovery}

In recent years, causal discovery methods have attracted attention from researchers owing to their ability to infer causal relationships from the data~\cite{Vowels2022causaldiscoverysurvey}. Among these, a large number of methods are dedicated to time-series data with applications in various domains such as healthcare, manufacturing, and energy~\cite{Assaad2022causaltimesurvey}. Below, we describe some representative causal discovery methods that are commonly used in causal inference-based RCA for microservice systems with metrics data. Furthermore, we also include a recent proposed causal discovery method, which is not yet explored in RCA literature.

\textbf{Granger Algorithm~\cite{Granger1980causal}.} The Granger algorithm is based on the concept of \textit{Granger causality}, which assumes that a time series causes another time series if the former provides statistically significant information about the future values of the latter. To derive the dependency between two time series $x$ and $y$, two autoregression models are constructed: one fitted using $y$ and one fitted using both $x$ and $y$. Then, a statistical test is performed to see if the predictions of $y$ that are based on past values of $x$ and $y$ are better than the predictions of $y$ that are based on its own past values.

\textbf{Peter-Clark (PC) Algorithm \cite{Spirtes1993Causal}.} The PC algorithm is one of the most popular causal discovery methods for time series data. It starts with a complete undirected graph and then checks for the dependencies and conditional independencies for all pairs of nodes to generate an undirected graph (\textit{skeleton graph}). Finally, a series of rules \cite{Spirtes1993Causal} is applied to the skeleton graph to orient the direction of the undirected edges. Developed from the PC algorithm, the PCMCI algorithm \cite{Runge2019PCMCI} is able to work with time-lagged causal relations and has also been shown to be effective.

\textbf{Fast Causal Inference (FCI) Algorithm \cite{Spirtes1993Causal}.} Similar to the PC algorithm, the FCI algorithm starts with an undirected graph and then sequentially removes the independent or conditionally independent edges with its set of rules. These rules are designed to ensure the FCI algorithm gives asymptotically correct causal graphs even in the presence of confounders. This is an advantage over the PC algorithm, as PC assumes there are no confounding factors that affect the time series. 

\textbf{LiNGAM Algorithm \cite{Shimizu2006Lingam}.} The LiNGAM algorithm formulates the relationships between the time series using a linear and acyclic structural equation model with non-Gaussian errors. The causal relationships between the time series can be inferred by checking whether the residuals and predictors of the structural equation model are independent. Similar to PC, LiNGAM also assumes there are no hidden confounders affecting the time series. There are two popular types of LiNGAM: ICALiNGAM~\cite{Shimizu2006Lingam}, which employs the independent component analysis, and DirectLiNGAM~\cite{Shimizu2011}, which uses regression analysis to build the structural equation model. 

\textbf{Greedy Equivalence Search (GES) Algorithm \cite{Chickering2002Ges}.} The GES algorithm starts with a graph without edges and greedily and sequentially adds the edges and their directions in a way that minimizes the Bayesian Information Score (BIC) \cite{Schwarz1978bic} or the Z score of hypothesis testing. Built on this base method, FGES (Fast GES)~\cite{Ramsey2017fges} constructs the causal graph in a way that is similar to FCI, i.e., relying on the collider causal structure when orienting the edges, making it more computationally efficient.

\textbf{NOTEARS-Low-Rank (NTLR) Algorithm \cite{fang2023low}.} NTLR is a gradient-based causal discovery method that extends NOTEARS~\cite{zheng2018dags} with low-rank graphs. Leveraging the low-rank assumption and existing techniques, NTLR adapts causal structure learning methods to offer several useful insights into interpretable graphical conditions. It also introduces novel adaptations addressing scenarios where traditional methods may encounter limitations.

\section{Detailed Information about Datasets}

\vspace{0.2cm}
\subsection{Synthetic Datasets} \label{sec:app-synthetic-dataset}

As discussed in Section \ref{sec:synthetic-data}, in this evaluation study, we use three different synthetic data generators of three previous RCA studies: CIRCA, RCD and CausIL \cite{Li2022Circa, Azam2022rcd, Chakraborty2023CausIL} to create synthetic datasets. These data generators are used in various research works to evaluate RCA methods for microservice systems \cite{Azam2022rcd, Li2022Circa, Chakraborty2023CausIL, liu2023pyrca}. The detailed information of these three synthetic dataset generators is as follows.

The synthetic data generator in~\cite{Li2022Circa} (CIRCA data generator) generates a random causal directed acyclic graph (DAG) based on a given number of nodes and edges. From the DAG, the time series data of each node is generated using a vector auto-regression (VAR) model. A fault is injected into a node by altering the noise item in the VAR model for 2 timestamps. The synthetic data generator in~\cite{Azam2022rcd} (RCD data generator) uses the pyAgrum package \cite{pyagrum} to generate a random DAG based on a given number of nodes and then draw time series data for each node. A fault is injected into a node by changing its conditional probability distribution. Note that for the RCD data generator, the time series data is discrete (values are integers from 0 to 5). The synthetic data generator in~\cite{Chakraborty2023CausIL} (CausIL data generator) generates the causal graphs and time series data in a way that mimics the behaviour of microservice systems. It considers that each service has 5 metrics: workload, CPU utilization, memory utilization, latency, and error count. It first constructs a DAG of services, then uses real metrics data to learn the metrics' characteristics, and from there, generates data for each node of the DAG. Finally, it is worth noting that, unlike CIRCA and RCD data generators, the CausIL data generator does not have the ability to inject faults, so there are no faulty datasets in our study created by the CausIL data generator.

We combine all three existing dataset generators to complement each other weaknesses, e.g. diverse causal graph structure, and metrics data types (continuous, discrete), to evaluate the performance of causal graph construction and causal inference-based RCA. % To the best of our knowledge, we are also the first to employ all three popular benchmark microservice systems, namely Online Boutique, Sock Shop, and large-scale Train Ticket, to generate datasets for RCA evaluation. Previous works \cite{yu2023nezha, Arya2021evalcausalai, Wang2021evalcausal, Azam2022rcd, Xin2023CausalRCA, Jinjin2018Microscope, Ma2020Automap, yu2021microrank, Wu2021Microdiag}, often employ one or two benchmark microservice systems, thus limiting their evaluation of the RCA methods. For example, large-scale Train-Ticket has 64 services but is mostly implemented in Java only, Online Boutique and Sock-Shop are implemented in many programming languages (e.g. Python, Go, C\#, and Javascript), but only have from 12 to 15 services. Our datasets are derived from all these systems, helping to evaluate diverse microservice systems from small-scale to large-scale. In summary, our datasets are significantly more diverse and comprehensive compared to previous works, helping us to mitigate the data limitations of previous works and discover new valuable insights.

\subsection{Benchmark Microservice Systems} \label{sec:app-microservice-system}

In this evaluation study, as described in Section \ref{sec:realworld-data}, we use three popular benchmark microservice systems, namely Sock Shop \cite{sockshop}, Online Boutique \cite{ob}, and Train Ticket \cite{tt}. 

Sock Shop \cite{sockshop} is a sock-selling e-commerce application that consists of 15 services communicating with each other through HTTP requests. Online Boutique \cite{ob}, which has 12 services, is an e-commerce application where users can browse items, add them to the cart and purchase them. Train Ticket \cite{tt} is one of the largest microservice systems simulating a train ticket booking system with 64 services. Compared to Sock Shop and Online Boutique, Train Ticket has longer and more complex failure propagation paths. These benchmark microservice systems have been widely recognized in previous works \cite{Jinjin2018Microscope, Azam2022rcd, Wu2021Microdiag, Xin2023CausalRCA, wu2022automatic, he2022graph, dan2021practical, yu2021microrank, zhou2018trainticket, Wang2021evalcausal}.

The way we deploy the three microservice systems, along with the monitoring system, is described in Section \ref{sec:realworld-data}. We then inject five common faults: CPU hog, memory leak, disk IO stress, network delay, and packet loss into several major services within the benchmark microservice systems. Specifically, we run the Online Boutique, Sock Shop, and Train Ticket applications for ten minutes to collect metrics data of the systems in the normal state. Next, we inject five faults into five targeted services of Online Boutique (adservice, cartservice, checkoutservice, currencyservice, and productcatalogue), five targeted services of Sock Shop (carts, catalogue, orders, payment, and user) and five targeted services of Train Ticket (ts-auth-service, ts-order-service, ts-route-service, ts-train-service, and ts-travel-service), and repeat the operation five times, yielding 125 cases for each benchmark system. We select these services as they are critical (their performance issues can affect other services). 

To ensure the independence of different injection operations, we restart the microservice systems after each experiment of injecting failures and collecting data instead of waiting for a cold down like~\cite{Wu2021Microdiag, yu2021microrank, Xin2023CausalRCA}. All the datasets we collect and use are publicly available at \url{https://anonymous.4open.science/r/ase24-cfm}.

\section{Hyperparameter Tuning} \label{sec:app-hyperpara-tuning}

In Section \ref{sec:rq1-results}, when evaluating the performance of causal discovery methods, apart from using default values of the hyperparameters, we also evaluate these methods with tuned hyperparameters. To tune the hyperparameters, we use the Bayesian Information Criterion (BIC) score \cite{Schwarz1978bic, biza2020bictuning} with cross-validation. Specifically, we first split all the metrics data into 2 parts: 2/3 for training and 1/3 for evaluation. We then create a search space consisting of multiple combinations of hyperparameters. For each combination, we run the causal discovery method on the training set and compute the BIC score on the evaluation set. Finally, we choose the combination of hyperparameters that yields the lowest BIC score (indicating better accuracy) and run the causal discovery method on the entire metrics data with this combination.

\section{Additional Experimental Results} \label{sec:app-additional-results}

\subsection{Efficiency of Causal Discovery Methods} In Section \ref{sec:efficency}, we evaluate how efficient causal discovery and RCA methods are. Here, Table A1 reports the running time (in seconds) of eight representative causal discovery methods on all six synthetic datasets. This is to answer the first part of the evaluation in Section \ref{sec:efficency}, which is to evaluate the efficiency of causal discovery methods.

\begin{table*}[!ht]
\centering

{\textbf{Table A1.} Running time (in seconds) of nine causal discovery algorithms on synthetic datasets in default settings.}

\label{table:q3-causal-speed}
\resizebox{0.65\textwidth}{!}{%
\begin{tabular}{l|r|r|r|r|r|r}
\hline
 & CIRCA10 & RCD10 & CausIL10 & CIRCA50 & RCD50 & CausIL50 \\ \hline \hline
PC & 0.38 & 0.27 & 0.3 & 3.47 & 2.01 & 38.6 \\ \hline
FCI & 0.51 & 0.28 & 0.3 & 8.19 & 2.32 & 336.6 \\ \hline
Granger & 1.95 & 2.53 & 4.4 & 70.78 & 57.09 & 118.8 \\ \hline
ICALiNGAM & 0.75 & 0.33 & 0.6 & 13.58 & 2.3 & 16.1 \\ \hline
DirectLiNGAM & 0.63 & 0.51 & 0.7 & 32.13 & 26.65 & 41.8 \\ \hline
GES & 3.24 & 0.58 & 4.6 & 84813$^*$ & 136.19 & 5543.5$^{**}$ \\ \hline
fGES & 1.92 & 0.37 & 2.2 & 34.42 & 5.28 & 67.4 \\ \hline
PCMCI & 4.8 & 5.95 & 17.2 & 255.25 & 542.77 & 1052.7 \\ \hline
NTLR & 45.53 & 14.49 & 368.1 & 932.61 & - & 2406.42 \\ \hline
\end{tabular}%
}

{\footnotesize \textit{ 
(*) results are reported from 1 case, which takes nearly 24 hours.\\ (**) results are partially obtained from 2/100 cases due to exceeding the 1 hour/case time-out constraint for 2 consecutive times (1h20m and 1h40m, respectively)}. 
}
\end{table*}

\subsection{Performance of Causal Discovery and RCA Methods with Different Input Data Lengths}

In Section \ref{sec:eval-input-data}, we evaluate the performance of the causal discovery and RCA methods with different input data lengths.

First, we show Figure A2, which reports the performance of six causal discovery methods (Granger, PC, FCI, ICALiNGAM, PCMCI and fGES) on the six synthetic datasets with input data lengths varying from 125 to 4000 data points. This figure is used to answer the first part of this evaluation, which is to evaluate how causal discovery methods perform with different input data lengths.

\begin{figure*}[!ht]
\centering
\includegraphics[width=\textwidth]{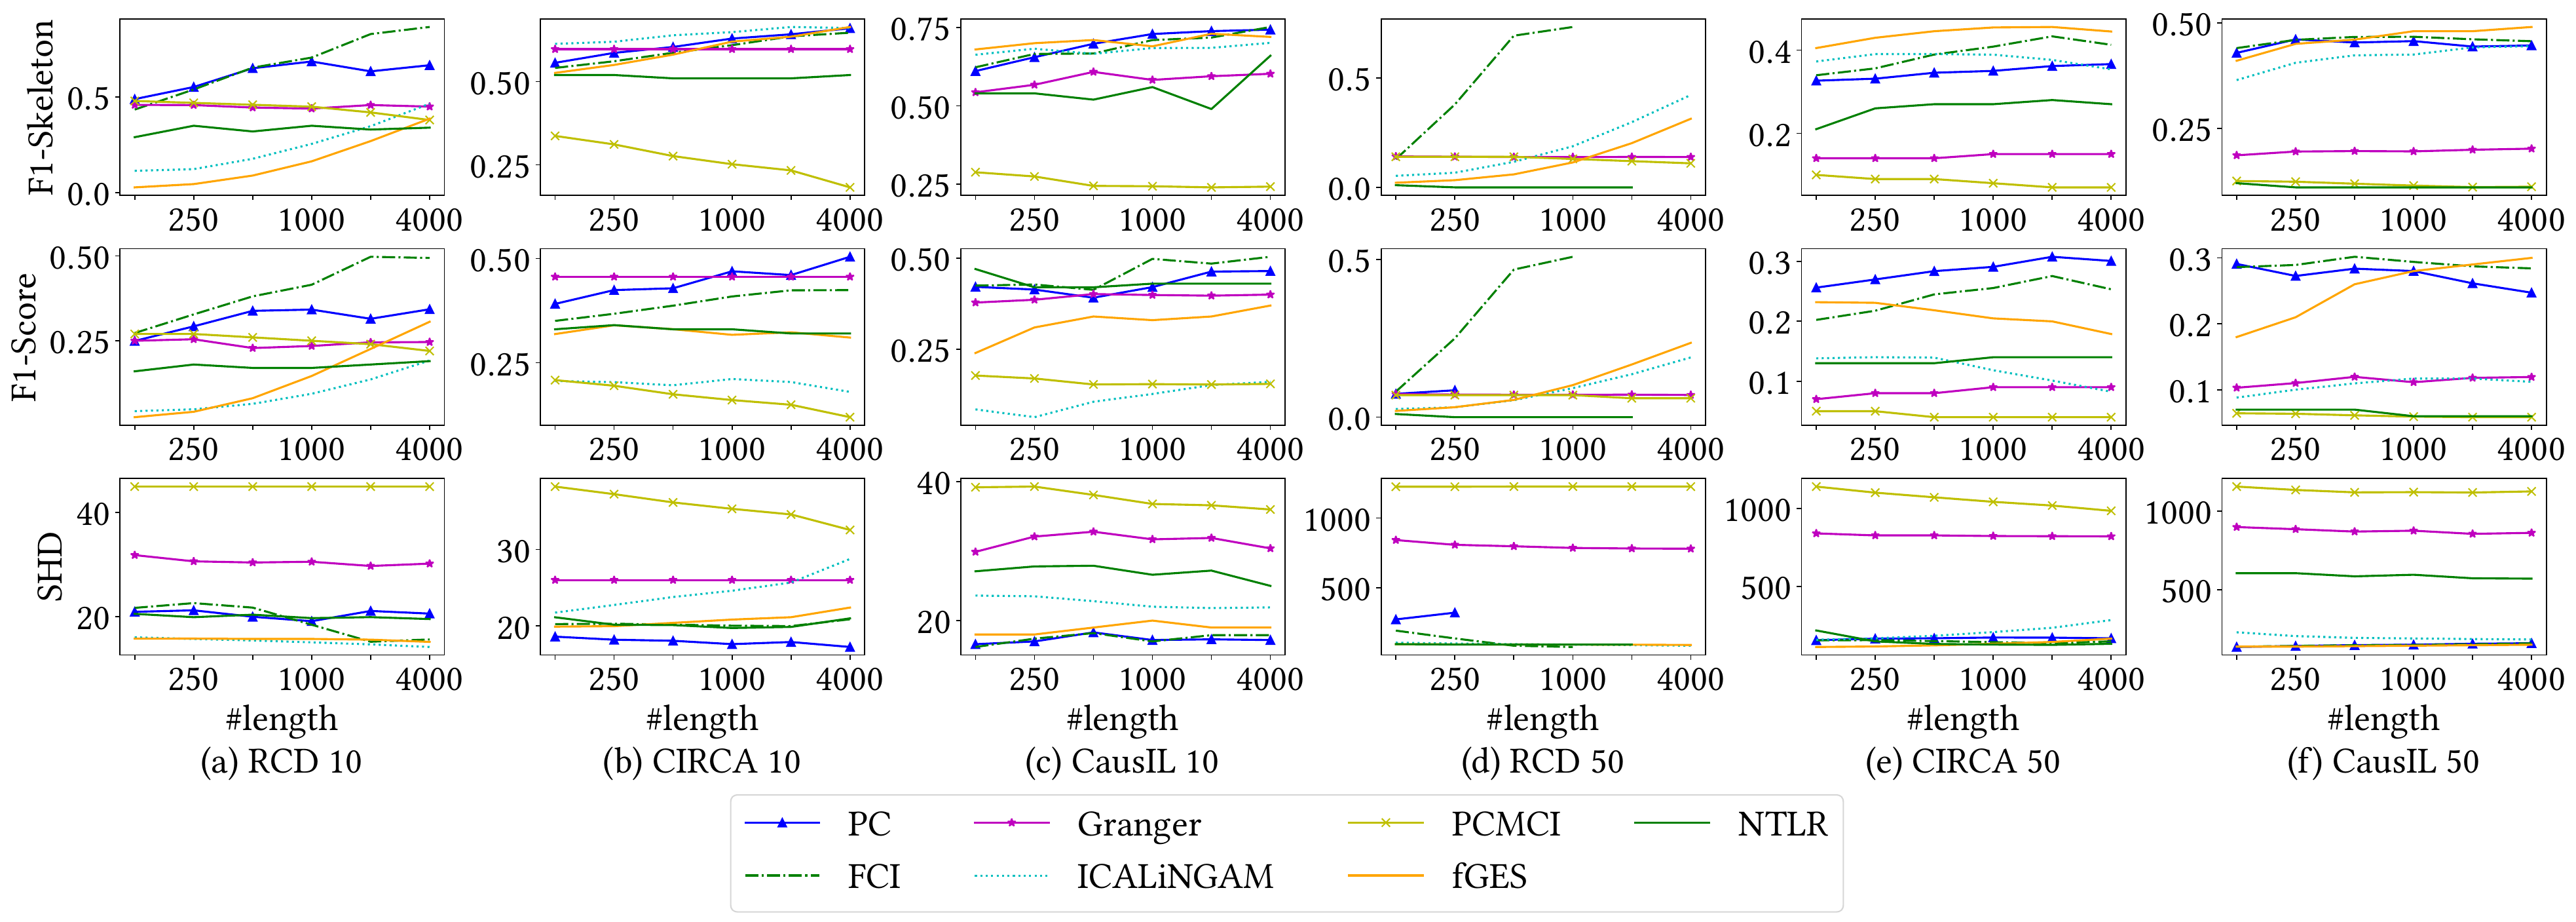}

{\footnotesize \textit{(*) PC, FCI, and NTLR results on RCD50 were partially obtained due to OOM errors during execution and exceeding the time limit.}} 

{\textbf{Figure A2.} Performance of seven causal discovery methods on six synthetic datasets with different data lengths.

A log-scale is used for the x-axis~\cite{Assaad2022causaltimesurvey}.}
\end{figure*}

Finally, we show Figure A3, which reports the performance of seven RCA methods on eight different datasets with input data lengths from 60 to 600 data points. This figure is used to answer the second part of the evaluation, which is to evaluate how RCA methods perform with different input data lengths.
